# Supplementary material for: Online Binary Models are Promising for Distinguishing Temporally Consistent Computer Usage Profiles
Source: arXiv:2105.09900 source file (2021-09-02)
Supplement: Supplementary file 1 [file appendix.tex]

\captionsetup[subfigure]{labelformat=empty, labelsep=colon}

\begin{figure}[htb]
    \centering
    \begin{subfigure}[b]{0.14\textwidth}
        \includegraphics[width=\textwidth]{figs/users_week/0101.png}
        \caption{Week 1.}
        \label{fig:user_week_0101}
    \end{subfigure}
    ~ %add desired spacing between images, e. g. ~, \quad, \qquad, \hfill etc. 
      %(or a blank line to force the subfigure onto a new line)
    \begin{subfigure}[b]{0.14\textwidth}
        \includegraphics[width=\textwidth]{figs/users_week/0102.png}
        \caption{Week 2.}
        \label{fig:user_week_0102}
    \end{subfigure}
    ~ %add desired spacing between images, e. g. ~, \quad, \qquad, \hfill etc. 
    %(or a blank line to force the subfigure onto a new line)
    \begin{subfigure}[b]{0.14\textwidth}
        \includegraphics[width=\textwidth]{figs/users_week/0103.png}
        \caption{Week 3.}
        \label{fig:user_week_0103}
    \end{subfigure}
    \caption{SOM images week-by-week for User 1.}
    \label{fig:user_week_01}
\end{figure}

\begin{figure}[htb]
    \centering
    \begin{subfigure}[b]{0.14\textwidth}
        \includegraphics[width=\textwidth]{figs/users_week/0201.png}
        \caption{Week 1.}
        \label{fig:user_week_0201}
    \end{subfigure}
    ~ %add desired spacing between images, e. g. ~, \quad, \qquad, \hfill etc. 
      %(or a blank line to force the subfigure onto a new line)
    \begin{subfigure}[b]{0.14\textwidth}
        \includegraphics[width=\textwidth]{figs/users_week/0202.png}
        \caption{Week 2.}
        \label{fig:user_week_0202}
    \end{subfigure}
    ~ %add desired spacing between images, e. g. ~, \quad, \qquad, \hfill etc. 
    %(or a blank line to force the subfigure onto a new line)
    \begin{subfigure}[b]{0.14\textwidth}
        \includegraphics[width=\textwidth]{figs/users_week/0203.png}
        \caption{Week 3.}
        \label{fig:user_week_0203}
    \end{subfigure}
    \caption{SOM images week-by-week for User 2.}
    \label{fig:user_week_02}
\end{figure}

\begin{figure}[htb]
    \centering
    \begin{subfigure}[b]{0.14\textwidth}
        \includegraphics[width=\textwidth]{figs/users_week/0301.png}
        \caption{Week 1.}
        \label{fig:user_week_0301}
    \end{subfigure}
    ~ %add desired spacing between images, e. g. ~, \quad, \qquad, \hfill etc. 
      %(or a blank line to force the subfigure onto a new line)
    \begin{subfigure}[b]{0.14\textwidth}
        \includegraphics[width=\textwidth]{figs/users_week/0302.png}
        \caption{Week 2.}
        \label{fig:user_week_0302}
    \end{subfigure}
    ~ %add desired spacing between images, e. g. ~, \quad, \qquad, \hfill etc. 
    %(or a blank line to force the subfigure onto a new line)
    \begin{subfigure}[b]{0.14\textwidth}
        \includegraphics[width=\textwidth]{figs/users_week/0303.png}
        \caption{Week 3.}
        \label{fig:user_week_0303}
    \end{subfigure}
    \caption{SOM images week-by-week for User 3.}
    \label{fig:user_week_03}
\end{figure}

\begin{figure}[htb]
    \centering
    \begin{subfigure}[b]{0.14\textwidth}
        \includegraphics[width=\textwidth]{figs/users_week/0401.png}
        \caption{Week 1.}
        \label{fig:user_week_0401}
    \end{subfigure}
    ~ %add desired spacing between images, e. g. ~, \quad, \qquad, \hfill etc. 
      %(or a blank line to force the subfigure onto a new line)
    \begin{subfigure}[b]{0.14\textwidth}
        \includegraphics[width=\textwidth]{figs/users_week/0402.png}
        \caption{Week 2.}
        \label{fig:user_week_0402}
    \end{subfigure}
    ~ %add desired spacing between images, e. g. ~, \quad, \qquad, \hfill etc. 
    %(or a blank line to force the subfigure onto a new line)
    \begin{subfigure}[b]{0.14\textwidth}
        \includegraphics[width=\textwidth]{figs/users_week/0403.png}
        \caption{Week 3.}
        \label{fig:user_week_0403}
    \end{subfigure}
    \caption{SOM images week-by-week for User 4.}
    \label{fig:user_week_04}
\end{figure}

\begin{figure}[htb]
    \centering
    \begin{subfigure}[b]{0.14\textwidth}
        \includegraphics[width=\textwidth]{figs/users_week/0501.png}
        \caption{Week 1.}
        \label{fig:user_week_0501}
    \end{subfigure}
    ~ %add desired spacing between images, e. g. ~, \quad, \qquad, \hfill etc. 
      %(or a blank line to force the subfigure onto a new line)
    \begin{subfigure}[b]{0.14\textwidth}
        \includegraphics[width=\textwidth]{figs/users_week/0502.png}
        \caption{Week 2.}
        \label{fig:user_week_0502}
    \end{subfigure}
    ~ %add desired spacing between images, e. g. ~, \quad, \qquad, \hfill etc. 
    %(or a blank line to force the subfigure onto a new line)
    \begin{subfigure}[b]{0.14\textwidth}
        \includegraphics[width=\textwidth]{figs/users_week/0503.png}
        \caption{Week 3.}
        \label{fig:user_week_0503}
    \end{subfigure}
    \caption{SOM images week-by-week for User 5.}
    \label{fig:user_week_05}
\end{figure}

\begin{figure}[htb]
    \centering
    \begin{subfigure}[b]{0.14\textwidth}
        \includegraphics[width=\textwidth]{figs/users_week/0601.png}
        \caption{Week 1.}
        \label{fig:user_week_0601}
    \end{subfigure}
    ~ %add desired spacing between images, e. g. ~, \quad, \qquad, \hfill etc. 
      %(or a blank line to force the subfigure onto a new line)
    \begin{subfigure}[b]{0.14\textwidth}
        \includegraphics[width=\textwidth]{figs/users_week/0602.png}
        \caption{Week 2.}
        \label{fig:user_week_0602}
    \end{subfigure}
    ~ %add desired spacing between images, e. g. ~, \quad, \qquad, \hfill etc. 
    %(or a blank line to force the subfigure onto a new line)
    \begin{subfigure}[b]{0.14\textwidth}
        \includegraphics[width=\textwidth]{figs/users_week/0603.png}
        \caption{Week 3.}
        \label{fig:user_week_0603}
    \end{subfigure}
    \caption{SOM images week-by-week for User 6.}
    \label{fig:user_week_06}
\end{figure}

\begin{figure}[htb]
    \centering
    \begin{subfigure}[b]{0.14\textwidth}
        \includegraphics[width=\textwidth]{figs/users_week/0701.png}
        \caption{Week 1.}
        \label{fig:user_week_0701}
    \end{subfigure}
    ~ %add desired spacing between images, e. g. ~, \quad, \qquad, \hfill etc. 
      %(or a blank line to force the subfigure onto a new line)
    \begin{subfigure}[b]{0.14\textwidth}
        \includegraphics[width=\textwidth]{figs/users_week/0702.png}
        \caption{Week 2.}
        \label{fig:user_week_0702}
    \end{subfigure}
    ~ %add desired spacing between images, e. g. ~, \quad, \qquad, \hfill etc. 
    %(or a blank line to force the subfigure onto a new line)
    \begin{subfigure}[b]{0.14\textwidth}
        \includegraphics[width=\textwidth]{figs/users_week/0703.png}
        \caption{Week 3.}
        \label{fig:user_week_0703}
    \end{subfigure}
    \caption{SOM images week-by-week for User 7.}
    \label{fig:user_week_07}
\end{figure}

\begin{figure}[htb]
    \centering
    \begin{subfigure}[b]{0.14\textwidth}
        \includegraphics[width=\textwidth]{figs/users_week/0801.png}
        \caption{Week 1.}
        \label{fig:user_week_0801}
    \end{subfigure}
    ~ %add desired spacing between images, e. g. ~, \quad, \qquad, \hfill etc. 
      %(or a blank line to force the subfigure onto a new line)
    \begin{subfigure}[b]{0.14\textwidth}
        \includegraphics[width=\textwidth]{figs/users_week/0802.png}
        \caption{Week 2.}
        \label{fig:user_week_0802}
    \end{subfigure}
    ~ %add desired spacing between images, e. g. ~, \quad, \qquad, \hfill etc. 
    %(or a blank line to force the subfigure onto a new line)
    \begin{subfigure}[b]{0.14\textwidth}
        \includegraphics[width=\textwidth]{figs/users_week/0803.png}
        \caption{Week 3.}
        \label{fig:user_week_0803}
    \end{subfigure}
    \caption{SOM images week-by-week for User 8.}
    \label{fig:user_week_08}
\end{figure}

\begin{figure}[htb]
    \centering
    \begin{subfigure}[b]{0.14\textwidth}
        \includegraphics[width=\textwidth]{figs/users_week/0901.png}
        \caption{Week 1.}
        \label{fig:user_week_0901}
    \end{subfigure}
    ~ %add desired spacing between images, e. g. ~, \quad, \qquad, \hfill etc. 
      %(or a blank line to force the subfigure onto a new line)
    \begin{subfigure}[b]{0.14\textwidth}
        \includegraphics[width=\textwidth]{figs/users_week/0902.png}
        \caption{Week 2.}
        \label{fig:user_week_0902}
    \end{subfigure}
    ~ %add desired spacing between images, e. g. ~, \quad, \qquad, \hfill etc. 
    %(or a blank line to force the subfigure onto a new line)
    \begin{subfigure}[b]{0.14\textwidth}
        \includegraphics[width=\textwidth]{figs/users_week/0903.png}
        \caption{Week 3.}
        \label{fig:user_week_0903}
    \end{subfigure}
    \caption{SOM images week-by-week for User 9.}
    \label{fig:user_week_09}
\end{figure}

\begin{figure}[htb]
    \centering
    \begin{subfigure}[b]{0.14\textwidth}
        \includegraphics[width=\textwidth]{figs/users_week/1001.png}
        \caption{Week 1.}
        \label{fig:user_week_1001}
    \end{subfigure}
    ~ %add desired spacing between images, e. g. ~, \quad, \qquad, \hfill etc. 
      %(or a blank line to force the subfigure onto a new line)
    \begin{subfigure}[b]{0.14\textwidth}
        \includegraphics[width=\textwidth]{figs/users_week/1002.png}
        \caption{Week 2.}
        \label{fig:user_week_1002}
    \end{subfigure}
    ~ %add desired spacing between images, e. g. ~, \quad, \qquad, \hfill etc. 
    %(or a blank line to force the subfigure onto a new line)
    \begin{subfigure}[b]{0.14\textwidth}
        \includegraphics[width=\textwidth]{figs/users_week/1003.png}
        \caption{Week 3.}
        \label{fig:user_week_1003}
    \end{subfigure}
    \caption{SOM images week-by-week for User 10.}
    \label{fig:user_week_10}
\end{figure}

\begin{figure}[htb]
    \centering
    \begin{subfigure}[b]{0.14\textwidth}
        \includegraphics[width=\textwidth]{figs/users_week/1101.png}
        \caption{Week 1.}
        \label{fig:user_week_1101}
    \end{subfigure}
    ~ %add desired spacing between images, e. g. ~, \quad, \qquad, \hfill etc. 
      %(or a blank line to force the subfigure onto a new line)
    \begin{subfigure}[b]{0.14\textwidth}
        \includegraphics[width=\textwidth]{figs/users_week/1102.png}
        \caption{Week 2.}
        \label{fig:user_week_1102}
    \end{subfigure}
    ~ %add desired spacing between images, e. g. ~, \quad, \qquad, \hfill etc. 
    %(or a blank line to force the subfigure onto a new line)
    \begin{subfigure}[b]{0.14\textwidth}
        \includegraphics[width=\textwidth]{figs/users_week/1103.png}
        \caption{Week 3.}
        \label{fig:user_week_1103}
    \end{subfigure}
    \caption{SOM images week-by-week for User 11.}
    \label{fig:user_week_11}
\end{figure}

\begin{figure}[htb]
    \centering
    \begin{subfigure}[b]{0.14\textwidth}
        \includegraphics[width=\textwidth]{figs/users_week/1201.png}
        \caption{Week 1.}
        \label{fig:user_week_1201}
    \end{subfigure}
    ~ %add desired spacing between images, e. g. ~, \quad, \qquad, \hfill etc. 
      %(or a blank line to force the subfigure onto a new line)
    \begin{subfigure}[b]{0.14\textwidth}
        \includegraphics[width=\textwidth]{figs/users_week/1202.png}
        \caption{Week 2.}
        \label{fig:user_week_1202}
    \end{subfigure}
    ~ %add desired spacing between images, e. g. ~, \quad, \qquad, \hfill etc. 
    %(or a blank line to force the subfigure onto a new line)
    \begin{subfigure}[b]{0.14\textwidth}
        \includegraphics[width=\textwidth]{figs/users_week/1203.png}
        \caption{Week 3.}
        \label{fig:user_week_1203}
    \end{subfigure}
    \caption{SOM images week-by-week for User 12.}
    \label{fig:user_week_12}
\end{figure}

\begin{figure}[ht]
    \centering
    \begin{subfigure}[b]{0.14\textwidth}
        \includegraphics[width=\textwidth]{figs/users_week/1301.png}
        \caption{Week 1.}
        \label{fig:user_week_1301}
    \end{subfigure}
    ~ %add desired spacing between images, e. g. ~, \quad, \qquad, \hfill etc. 
      %(or a blank line to force the subfigure onto a new line)
    \begin{subfigure}[b]{0.14\textwidth}
        \includegraphics[width=\textwidth]{figs/users_week/1302.png}
        \caption{Week 2.}
        \label{fig:user_week_1302}
    \end{subfigure}
    ~ %add desired spacing between images, e. g. ~, \quad, \qquad, \hfill etc. 
    %(or a blank line to force the subfigure onto a new line)
    \begin{subfigure}[b]{0.14\textwidth}
        \includegraphics[width=\textwidth]{figs/users_week/1303.png}
        \caption{Week 3.}
        \label{fig:user_week_1303}
    \end{subfigure}
    \caption{SOM images week-by-week for User 13.}
    \label{fig:user_week_13}
\end{figure}

\begin{figure}[ht]
    \centering
    \begin{subfigure}[b]{0.14\textwidth}
        \includegraphics[width=\textwidth]{figs/users_week/1401.png}
        \caption{Week 1.}
        \label{fig:user_week_1401}
    \end{subfigure}
    ~ %add desired spacing between images, e. g. ~, \quad, \qquad, \hfill etc. 
      %(or a blank line to force the subfigure onto a new line)
    \begin{subfigure}[b]{0.14\textwidth}
        \includegraphics[width=\textwidth]{figs/users_week/1402.png}
        \caption{Week 2.}
        \label{fig:user_week_1402}
    \end{subfigure}
    ~ %add desired spacing between images, e. g. ~, \quad, \qquad, \hfill etc. 
    %(or a blank line to force the subfigure onto a new line)
    \begin{subfigure}[b]{0.14\textwidth}
        \includegraphics[width=\textwidth]{figs/users_week/1403.png}
        \caption{Week 3.}
        \label{fig:user_week_1403}
    \end{subfigure}
    \caption{SOM images week-by-week for User 14.}
    \label{fig:user_week_14}
\end{figure}

\begin{figure}[ht]
    \centering
    \begin{subfigure}[b]{0.14\textwidth}
        \includegraphics[width=\textwidth]{figs/users_week/1501.png}
        \caption{Week 1.}
        \label{fig:user_week_1501}
    \end{subfigure}
    ~ %add desired spacing between images, e. g. ~, \quad, \qquad, \hfill etc. 
      %(or a blank line to force the subfigure onto a new line)
    \begin{subfigure}[b]{0.14\textwidth}
        \includegraphics[width=\textwidth]{figs/users_week/1502.png}
        \caption{Week 2.}
        \label{fig:user_week_1502}
    \end{subfigure}
    ~ %add desired spacing between images, e. g. ~, \quad, \qquad, \hfill etc. 
    %(or a blank line to force the subfigure onto a new line)
    \begin{subfigure}[b]{0.14\textwidth}
        \includegraphics[width=\textwidth]{figs/users_week/1503.png}
        \caption{Week 3.}
        \label{fig:user_week_1503}
    \end{subfigure}
    \caption{SOM images week-by-week for User 15.}
    \label{fig:user_week_15}
\end{figure}

\begin{figure}[ht]
    \centering
    \begin{subfigure}[b]{0.14\textwidth}
        \includegraphics[width=\textwidth]{figs/users_week/1601.png}
        \caption{Week 1.}
        \label{fig:user_week_1601}
    \end{subfigure}
    ~ %add desired spacing between images, e. g. ~, \quad, \qquad, \hfill etc. 
      %(or a blank line to force the subfigure onto a new line)
    \begin{subfigure}[b]{0.14\textwidth}
        \includegraphics[width=\textwidth]{figs/users_week/1602.png}
        \caption{Week 2.}
        \label{fig:user_week_1602}
    \end{subfigure}
    ~ %add desired spacing between images, e. g. ~, \quad, \qquad, \hfill etc. 
    %(or a blank line to force the subfigure onto a new line)
    \begin{subfigure}[b]{0.14\textwidth}
        \includegraphics[width=\textwidth]{figs/users_week/1603.png}
        \caption{Week 3.}
        \label{fig:user_week_1603}
    \end{subfigure}
    \caption{SOM images week-by-week for User 16.}
    \label{fig:user_week_16}
\end{figure}

\begin{figure}[ht]
    \centering
    \begin{subfigure}[b]{0.14\textwidth}
        \includegraphics[width=\textwidth]{figs/users_week/1701.png}
        \caption{Week 1.}
        \label{fig:user_week_1701}
    \end{subfigure}
    ~ %add desired spacing between images, e. g. ~, \quad, \qquad, \hfill etc. 
      %(or a blank line to force the subfigure onto a new line)
    \begin{subfigure}[b]{0.14\textwidth}
        \includegraphics[width=\textwidth]{figs/users_week/1702.png}
        \caption{Week 2.}
        \label{fig:user_week_1702}
    \end{subfigure}
    ~ %add desired spacing between images, e. g. ~, \quad, \qquad, \hfill etc. 
    %(or a blank line to force the subfigure onto a new line)
    \begin{subfigure}[b]{0.14\textwidth}
        \includegraphics[width=\textwidth]{figs/users_week/1703.png}
        \caption{Week 3.}
        \label{fig:user_week_1703}
    \end{subfigure}
    \caption{SOM images week-by-week for User 17.}
    \label{fig:user_week_17}
\end{figure}

\begin{figure}[ht]
    \centering
    \begin{subfigure}[b]{0.14\textwidth}
        \includegraphics[width=\textwidth]{figs/users_week/1801.png}
        \caption{Week 1.}
        \label{fig:user_week_1801}
    \end{subfigure}
    ~ %add desired spacing between images, e. g. ~, \quad, \qquad, \hfill etc. 
      %(or a blank line to force the subfigure onto a new line)
    \begin{subfigure}[b]{0.14\textwidth}
        \includegraphics[width=\textwidth]{figs/users_week/1802.png}
        \caption{Week 2.}
        \label{fig:user_week_1802}
    \end{subfigure}
    ~ %add desired spacing between images, e. g. ~, \quad, \qquad, \hfill etc. 
    %(or a blank line to force the subfigure onto a new line)
    \begin{subfigure}[b]{0.14\textwidth}
        \includegraphics[width=\textwidth]{figs/users_week/1803.png}
        \caption{Week 3.}
        \label{fig:user_week_1803}
    \end{subfigure}
    \caption{SOM images week-by-week for User 18.}
    \label{fig:user_week_18}
    % \vspace{7.3in}
\end{figure}

% \begin{figure}[htb]
%     \begin{multicols}{3}
%         \centering
%         \subcaptionbox{Week 1.\label{fig:user_0101}}[\linewidth][c]{
%         \includegraphics[width=.14\textwidth]{figs/users_week/0101.png}}\par
%         \subcaptionbox{Week 2.\label{fig:user_0102}}[\linewidth][c]{
%         \includegraphics[width=.14\textwidth]{figs/users_week/0102.png}}\par
%         \subcaptionbox{Week 3.\label{fig:user_0103}}[\linewidth][c]{
%         \includegraphics[width=.14\textwidth]{figs/users_week/0103.png}}\par 
%     \end{multicols}
%     \caption{SOM images week-by-week for user 1.}
%     \label{fig:som_user_01}
% \end{figure}
% ~
% \begin{figure}[htb]
%     \begin{multicols}{3}
%         \centering
%         \subcaptionbox{Week 1.\label{fig:user_0201}}[\linewidth][c]{
%         \includegraphics[width=.14\textwidth]{figs/users_week/0201.png}}\par
%         \subcaptionbox{Week 2.\label{fig:user_0202}}[\linewidth][c]{
%         \includegraphics[width=.14\textwidth]{figs/users_week/0202.png}}\par
%         \subcaptionbox{Week 3.\label{fig:user_0203}}[\linewidth][c]{
%         \includegraphics[width=.14\textwidth]{figs/users_week/0203.png}}\par 
%     \end{multicols}
%     \caption{SOM images week-by-week for user 2.}
%     \label{fig:som_user_02}
% \end{figure}

% \begin{figure}[htb]
%     \begin{multicols}{3}
%         \centering
%         \subcaptionbox{Week 1.\label{fig:user_0301}}[\linewidth][c]{
%         \includegraphics[width=.14\textwidth]{figs/users_week/0301.png}}\par
%         \subcaptionbox{Week 2.\label{fig:user_0302}}[\linewidth][c]{
%         \includegraphics[width=.14\textwidth]{figs/users_week/0302.png}}\par
%         \subcaptionbox{Week 3.\label{fig:user_0303}}[\linewidth][c]{
%         \includegraphics[width=.14\textwidth]{figs/users_week/0303.png}}\par 
%     \end{multicols}
%     \caption{SOM images week-by-week for user 3.}
%     \label{fig:som_user_03}
% \end{figure}
% ~
% \begin{figure}[htb]
%     \begin{multicols}{3}
%         \centering
%         \subcaptionbox{Week 1.\label{fig:user_0401}}[\linewidth][c]{
%         \includegraphics[width=.14\textwidth]{figs/users_week/0401.png}}\par
%         \subcaptionbox{Week 2.\label{fig:user_0402}}[\linewidth][c]{
%         \includegraphics[width=.14\textwidth]{figs/users_week/0402.png}}\par
%         \subcaptionbox{Week 3.\label{fig:user_0403}}[\linewidth][c]{
%         \includegraphics[width=.14\textwidth]{figs/users_week/0403.png}}\par 
%     \end{multicols}
%     \caption{SOM images week-by-week for user 4.}
%     \label{fig:som_user_04}
% \end{figure}

% \begin{figure}[htb]
%     \begin{multicols}{3}
%         \centering
%         \subcaptionbox{Week 1.\label{fig:user_0501}}[\linewidth][c]{
%         \includegraphics[width=.14\textwidth]{figs/users_week/0501.png}}\par
%         \subcaptionbox{Week 2.\label{fig:user_0502}}[\linewidth][c]{
%         \includegraphics[width=.14\textwidth]{figs/users_week/0502.png}}\par
%         \subcaptionbox{Week 3.\label{fig:user_0503}}[\linewidth][c]{
%         \includegraphics[width=.14\textwidth]{figs/users_week/0503.png}}\par 
%     \end{multicols}
%     \caption{SOM images week-by-week for user 5.}
%     \label{fig:som_user_05}
% \end{figure}
% ~
% \begin{figure}[htb]
%     \begin{multicols}{3}
%         \centering
%         \subcaptionbox{Week 1.\label{fig:user_0601}}[\linewidth][c]{
%         \includegraphics[width=.14\textwidth]{figs/users_week/0601.png}}\par
%         \subcaptionbox{Week 2.\label{fig:user_0602}}[\linewidth][c]{
%         \includegraphics[width=.14\textwidth]{figs/users_week/0602.png}}\par
%         \subcaptionbox{Week 3.\label{fig:user_0603}}[\linewidth][c]{
%         \includegraphics[width=.14\textwidth]{figs/users_week/0603.png}}\par 
%     \end{multicols}
%     \caption{SOM images week-by-week for user 6.}
%     \label{fig:som_user_06}
% \end{figure}

% \begin{figure}[htb]
%     \begin{multicols}{3}
%         \centering
%         \subcaptionbox{Week 1.\label{fig:user_0701}}[\linewidth][c]{
%         \includegraphics[width=.14\textwidth]{figs/users_week/0701.png}}\par
%         \subcaptionbox{Week 2.\label{fig:user_0702}}[\linewidth][c]{
%         \includegraphics[width=.14\textwidth]{figs/users_week/0702.png}}\par
%         \subcaptionbox{Week 3.\label{fig:user_0703}}[\linewidth][c]{
%         \includegraphics[width=.14\textwidth]{figs/users_week/0703.png}}\par 
%     \end{multicols}
%     \caption{SOM images week-by-week for user 5.}
%     \label{fig:som_user_07}
% \end{figure}
% ~
% \begin{figure}[htb]
%     \begin{multicols}{3}
%         \centering
%         \subcaptionbox{Week 1.\label{fig:user_0801}}[\linewidth][c]{
%         \includegraphics[width=.14\textwidth]{figs/users_week/0801.png}}\par
%         \subcaptionbox{Week 2.\label{fig:user_0802}}[\linewidth][c]{
%         \includegraphics[width=.14\textwidth]{figs/users_week/0802.png}}\par
%         \subcaptionbox{Week 3.\label{fig:user_0803}}[\linewidth][c]{
%         \includegraphics[width=.14\textwidth]{figs/users_week/0803.png}}\par 
%     \end{multicols}
%     \caption{SOM images week-by-week for user 8.}
%     \label{fig:som_user_08}
% \end{figure}
